# Supplementary material for: Context-aware Learned Mesh-based Simulation via Trajectory-Level Meta-Learning
Source: arXiv:2511.05234 source file (2026-01-21)
Supplement: Supplementary file 1 [file ltsgns_all_tasks.tex]

\begin{figure*}
    \centering
    \begin{minipage}{0.12\textwidth}
            \centering
            \includegraphics[width=\textwidth]{03_appendix/timestep_figures/app_plate_ltsgns_step_0000.png}
            \caption*{$t=0$}
    \end{minipage}
    \begin{minipage}{0.12\textwidth}
            \centering
            \includegraphics[width=\textwidth]{03_appendix/timestep_figures/app_plate_ltsgns_step_0010.png}
            \caption*{$t=10$}
    \end{minipage}
    \begin{minipage}{0.12\textwidth}
            \centering
            \includegraphics[width=\textwidth]{03_appendix/timestep_figures/app_plate_ltsgns_step_0020.png}
            \caption*{$t=20$}
    \end{minipage}
    \begin{minipage}{0.12\textwidth}
            \centering
            \includegraphics[width=\textwidth]{03_appendix/timestep_figures/app_plate_ltsgns_step_0030.png}
            \caption*{$t=30$}
    \end{minipage}
    \begin{minipage}{0.12\textwidth}
            \centering
            \includegraphics[width=\textwidth]{03_appendix/timestep_figures/app_plate_ltsgns_step_0035.png}
            \caption*{$t=35$}
    \end{minipage}
    \begin{minipage}{0.12\textwidth}
            \centering
            \includegraphics[width=\textwidth]{03_appendix/timestep_figures/app_plate_ltsgns_step_0040.png}
            \caption*{$t=40$}
    \end{minipage}
    \begin{minipage}{0.12\textwidth}
            \centering
            \includegraphics[width=\textwidth]{03_appendix/timestep_figures/app_plate_ltsgns_step_0045.png}
            \caption*{$t=45$}
    \end{minipage}
    \begin{minipage}{0.12\textwidth}
            \centering
            \includegraphics[width=\textwidth]{03_appendix/timestep_figures/app_plate_ltsgns_step_0050.png}
            \caption*{$t=50$}
    \end{minipage}

        \begin{minipage}{0.12\textwidth}
            \centering
            \includegraphics[width=\textwidth]{03_appendix/timestep_figures/app_tissue_ltsgns_step_0000.png}
            \caption*{$t=0$}
    \end{minipage}
    \begin{minipage}{0.12\textwidth}
            \centering
            \includegraphics[width=\textwidth]{03_appendix/timestep_figures/app_tissue_ltsgns_step_0020.png}
            \caption*{$t=20$}
    \end{minipage}
    \begin{minipage}{0.12\textwidth}
            \centering
            \includegraphics[width=\textwidth]{03_appendix/timestep_figures/app_tissue_ltsgns_step_0040.png}
            \caption*{$t=40$}
    \end{minipage}
    \begin{minipage}{0.12\textwidth}
            \centering
            \includegraphics[width=\textwidth]{03_appendix/timestep_figures/app_tissue_ltsgns_step_0060.png}
            \caption*{$t=60$}
    \end{minipage}
    \begin{minipage}{0.12\textwidth}
            \centering
            \includegraphics[width=\textwidth]{03_appendix/timestep_figures/app_tissue_ltsgns_step_0070.png}
            \caption*{$t=70$}
    \end{minipage}
    \begin{minipage}{0.12\textwidth}
            \centering
            \includegraphics[width=\textwidth]{03_appendix/timestep_figures/app_tissue_ltsgns_step_0080.png}
            \caption*{$t=80$}
    \end{minipage}
    \begin{minipage}{0.12\textwidth}
            \centering
            \includegraphics[width=\textwidth]{03_appendix/timestep_figures/app_tissue_ltsgns_step_0090.png}
            \caption*{$t=90$}
    \end{minipage}
    \begin{minipage}{0.12\textwidth}
            \centering
            \includegraphics[width=\textwidth]{03_appendix/timestep_figures/app_tissue_ltsgns_step_0100.png}
            \caption*{$t=100$}
    \end{minipage}
    
    \begin{minipage}{0.12\textwidth}
            \centering
            \includegraphics[width=\textwidth]{03_appendix/timestep_figures/app_fig1_step_0030.png}
            \caption*{$t=30$}
    \end{minipage}
    \begin{minipage}{0.12\textwidth}
            \centering
            \includegraphics[width=\textwidth]{03_appendix/timestep_figures/app_fig1_step_0040.png}
            \caption*{$t=40$}
    \end{minipage}
    \begin{minipage}{0.12\textwidth}
            \centering
            \includegraphics[width=\textwidth]{03_appendix/timestep_figures/app_fig1_step_0050.png}
            \caption*{$t=50$}
    \end{minipage}
    \begin{minipage}{0.12\textwidth}
            \centering
            \includegraphics[width=\textwidth]{03_appendix/timestep_figures/app_fig1_step_0060.png}
            \caption*{$t=60$}
    \end{minipage}
    \begin{minipage}{0.12\textwidth}
            \centering
            \includegraphics[width=\textwidth]{03_appendix/timestep_figures/app_fig1_step_0070.png}
            \caption*{$t=70$}
    \end{minipage}
    \begin{minipage}{0.12\textwidth}
            \centering
            \includegraphics[width=\textwidth]{03_appendix/timestep_figures/app_fig1_step_0080.png}
            \caption*{$t=80$}
    \end{minipage}
    \begin{minipage}{0.12\textwidth}
            \centering
            \includegraphics[width=\textwidth]{03_appendix/timestep_figures/app_fig1_step_0090.png}
            \caption*{$t=90$}
    \end{minipage}
    \begin{minipage}{0.12\textwidth}
            \centering
            \includegraphics[width=\textwidth]{03_appendix/timestep_figures/app_fig1_step_0100.png}
            \caption*{$t=100$}
    \end{minipage}

        \begin{minipage}{0.12\textwidth}
            \centering
            \includegraphics[width=\textwidth]{03_appendix/timestep_figures/app_teddy_ltsgns_step_0000.png}
            \caption*{$t=0$}
    \end{minipage}
    \begin{minipage}{0.12\textwidth}
            \centering
            \includegraphics[width=\textwidth]{03_appendix/timestep_figures/app_teddy_ltsgns_step_0025.png}
            \caption*{$t=25$}
    \end{minipage}
    \begin{minipage}{0.12\textwidth}
            \centering
            \includegraphics[width=\textwidth]{03_appendix/timestep_figures/app_teddy_ltsgns_step_0050.png}
            \caption*{$t=50$}
    \end{minipage}
    \begin{minipage}{0.12\textwidth}
            \centering
            \includegraphics[width=\textwidth]{03_appendix/timestep_figures/app_teddy_ltsgns_step_0075.png}
            \caption*{$t=75$}
    \end{minipage}
    \begin{minipage}{0.12\textwidth}
            \centering
            \includegraphics[width=\textwidth]{03_appendix/timestep_figures/app_teddy_ltsgns_step_0100.png}
            \caption*{$t=100$}
    \end{minipage}
    \begin{minipage}{0.12\textwidth}
            \centering
            \includegraphics[width=\textwidth]{03_appendix/timestep_figures/app_teddy_ltsgns_step_0125.png}
            \caption*{$t=125$}
    \end{minipage}
    \begin{minipage}{0.12\textwidth}
            \centering
            \includegraphics[width=\textwidth]{03_appendix/timestep_figures/app_teddy_ltsgns_step_0150.png}
            \caption*{$t=150$}
    \end{minipage}
    \begin{minipage}{0.12\textwidth}
            \centering
            \includegraphics[width=\textwidth]{03_appendix/timestep_figures/app_teddy_ltsgns_step_0200.png}
            \caption*{$t=200$}
    \end{minipage}

    \begin{minipage}{0.12\textwidth}
            \centering
            \includegraphics[width=\textwidth]{03_appendix/timestep_figures/app_worm_ltsgns_step_0000.png}
            \caption*{$t=0$}
    \end{minipage}
    \begin{minipage}{0.12\textwidth}
            \centering
            \includegraphics[width=\textwidth]{03_appendix/timestep_figures/app_worm_ltsgns_step_0025.png}
            \caption*{$t=25$}
    \end{minipage}
    \begin{minipage}{0.12\textwidth}
            \centering
            \includegraphics[width=\textwidth]{03_appendix/timestep_figures/app_worm_ltsgns_step_0050.png}
            \caption*{$t=50$}
    \end{minipage}
    \begin{minipage}{0.12\textwidth}
            \centering
            \includegraphics[width=\textwidth]{03_appendix/timestep_figures/app_worm_ltsgns_step_0075.png}
            \caption*{$t=75$}
    \end{minipage}
    \begin{minipage}{0.12\textwidth}
            \centering
            \includegraphics[width=\textwidth]{03_appendix/timestep_figures/app_worm_ltsgns_step_0100.png}
            \caption*{$t=100$}
    \end{minipage}
    \begin{minipage}{0.12\textwidth}
            \centering
            \includegraphics[width=\textwidth]{03_appendix/timestep_figures/app_worm_ltsgns_step_0125.png}
            \caption*{$t=125$}
    \end{minipage}
    \begin{minipage}{0.12\textwidth}
            \centering
            \includegraphics[width=\textwidth]{03_appendix/timestep_figures/app_worm_ltsgns_step_0150.png}
            \caption*{$t=150$}
    \end{minipage}
    \begin{minipage}{0.12\textwidth}
            \centering
            \includegraphics[width=\textwidth]{03_appendix/timestep_figures/app_worm_ltsgns_step_0200.png}
            \caption*{$t=200$}
    \end{minipage}
    
    \vspace{0.01\textwidth}%

    \caption{
    Simulation over time of an exemplary test trajectory for~\gls{ltsgns} across different tasks.
    All visualizations show the \textbf{\textcolor{blue}{predicted mesh}}, a \textbf{\textcolor{darkgray}{collider or floor}}, a \textbf{\textcolor{orange}{wireframe}} of the ground-truth simulation, and \textbf{\textcolor{purple}{correspondences}} between predicted and ground truth vertices.
    \gls{ltsgns} provides accurate physical simulations for up to $200$ time steps.
    }
    \label{fig:appendix_results_all_tasks}
\end{figure*}
