# Supplementary material for: Context-aware Learned Mesh-based Simulation via Trajectory-Level Meta-Learning
Source: arXiv:2511.05234 source file (2026-01-21)
Supplement: Supplementary file 2 [file mof_vm_all_methods.tex]

\begin{figure*}
    \centering
    \begin{minipage}{0.12\textwidth}
            \centering
            \includegraphics[width=\textwidth]{03_appendix/timestep_figures/app_pylon_ltsgns_step0000.png}
    \end{minipage}
    \begin{minipage}{0.12\textwidth}
            \centering
            \includegraphics[width=\textwidth]{03_appendix/timestep_figures/app_pylon_ltsgns_step0025.png}
    \end{minipage}
    \begin{minipage}{0.12\textwidth}
            \centering
            \includegraphics[width=\textwidth]{03_appendix/timestep_figures/app_pylon_ltsgns_step0050.png}
    \end{minipage}
    \begin{minipage}{0.12\textwidth}
            \centering
            \includegraphics[width=\textwidth]{03_appendix/timestep_figures/app_pylon_ltsgns_step0075.png}
    \end{minipage}
    \begin{minipage}{0.12\textwidth}
            \centering
            \includegraphics[width=\textwidth]{03_appendix/timestep_figures/app_pylon_ltsgns_step0100.png}
    \end{minipage}
    \begin{minipage}{0.12\textwidth}
            \centering
            \includegraphics[width=\textwidth]{03_appendix/timestep_figures/app_pylon_ltsgns_step0125.png}
    \end{minipage}
    \begin{minipage}{0.12\textwidth}
            \centering
            \includegraphics[width=\textwidth]{03_appendix/timestep_figures/app_pylon_ltsgns_step0150.png}
    \end{minipage}
    \begin{minipage}{0.12\textwidth}
            \centering
            \includegraphics[width=\textwidth]{03_appendix/timestep_figures/app_pylon_ltsgns_step0200.png}
    \end{minipage}

    \begin{minipage}{0.12\textwidth}
            \centering
            \includegraphics[width=\textwidth]{03_appendix/timestep_figures/app_pylon_mgn_step0000.png}
    \end{minipage}
    \begin{minipage}{0.12\textwidth}
            \centering
            \includegraphics[width=\textwidth]{03_appendix/timestep_figures/app_pylon_mgn_step0025.png}
    \end{minipage}
    \begin{minipage}{0.12\textwidth}
            \centering
            \includegraphics[width=\textwidth]{03_appendix/timestep_figures/app_pylon_mgn_step0050.png}
    \end{minipage}
    \begin{minipage}{0.12\textwidth}
            \centering
            \includegraphics[width=\textwidth]{03_appendix/timestep_figures/app_pylon_mgn_step0075.png}
    \end{minipage}
    \begin{minipage}{0.12\textwidth}
            \centering
            \includegraphics[width=\textwidth]{03_appendix/timestep_figures/app_pylon_mgn_step0100.png}
    \end{minipage}
    \begin{minipage}{0.12\textwidth}
            \centering
            \includegraphics[width=\textwidth]{03_appendix/timestep_figures/app_pylon_mgn_step0125.png}
    \end{minipage}
    \begin{minipage}{0.12\textwidth}
            \centering
            \includegraphics[width=\textwidth]{03_appendix/timestep_figures/app_pylon_mgn_step0150.png}
    \end{minipage}
    \begin{minipage}{0.12\textwidth}
            \centering
            \includegraphics[width=\textwidth]{03_appendix/timestep_figures/app_pylon_mgn_step0200.png}
    \end{minipage}

    \begin{minipage}{0.12\textwidth}
            \centering
            \includegraphics[width=\textwidth]{03_appendix/timestep_figures/app_pylon_mgn_oracle_step0000.png}
            \caption*{$t=0$}
    \end{minipage}
    \begin{minipage}{0.12\textwidth}
            \centering
            \includegraphics[width=\textwidth]{03_appendix/timestep_figures/app_pylon_mgn_oracle_step0025.png}
            \caption*{$t=25$}
    \end{minipage}
    \begin{minipage}{0.12\textwidth}
            \centering
            \includegraphics[width=\textwidth]{03_appendix/timestep_figures/app_pylon_mgn_oracle_step0050.png}
            \caption*{$t=50$}
    \end{minipage}
    \begin{minipage}{0.12\textwidth}
            \centering
            \includegraphics[width=\textwidth]{03_appendix/timestep_figures/app_pylon_mgn_oracle_step0075.png}
            \caption*{$t=75$}
    \end{minipage}
    \begin{minipage}{0.12\textwidth}
            \centering
            \includegraphics[width=\textwidth]{03_appendix/timestep_figures/app_pylon_mgn_oracle_step0100.png}
            \caption*{$t=100$}
    \end{minipage}
    \begin{minipage}{0.12\textwidth}
            \centering
            \includegraphics[width=\textwidth]{03_appendix/timestep_figures/app_pylon_mgn_oracle_step0125.png}
            \caption*{$t=125$}
    \end{minipage}
    \begin{minipage}{0.12\textwidth}
            \centering
            \includegraphics[width=\textwidth]{03_appendix/timestep_figures/app_pylon_mgn_oracle_step0150.png}
            \caption*{$t=150$}
    \end{minipage}
    \begin{minipage}{0.12\textwidth}
            \centering
            \includegraphics[width=\textwidth]{03_appendix/timestep_figures/app_pylon_mgn_oracle_step0200.png}
            \caption*{$t=200$}
    \end{minipage}

    \caption{
    Simulation over time of an exemplary test trajectory for \textbf{\textcolor{blue}{\gls{ltsgns}}}, \textbf{\textcolor{orange}{\gls{mgn}}} and \textbf{\textcolor{olive}{\gls{mgn} (Oracle)}} for the \textit{Mixed Object Fall (Varied Material)} task.
    All visualizations show the show the predicted mesh, a \textbf{\textcolor{darkgray}{collider or floor}}, a \textbf{\textcolor{orange}{wireframe}} of the ground-truth simulation, and \textbf{\textcolor{purple}{correspondences}} between predicted and ground truth vertices.
    Only \gls{ltsgns} closely matches the ground truth simulation.
    }
    \label{fig:appendix_results_mov_vm_all_methods}
\end{figure*}
