# Supplementary material for: Context-aware Learned Mesh-based Simulation via Trajectory-Level Meta-Learning
Source: arXiv:2511.05234 source file (2026-01-21)
Supplement: Supplementary file 3 [file mse_time_steps_mid_context.tex]

\begin{figure*}[t]
    \makebox[\textwidth][c]{
    \input{02_figures/legend/three_methods_nomarker}
    }
    \centering
    \begin{subfigure}[b]{0.49\linewidth} % Adjust the width as needed
        \includegraphics[width=\textwidth]{03_appendix/figure_matrix/mse_time_steps/deformable_plate_v2/mse_per_timestep_2fig_context_size_5.pdf}
        \caption{Deformable Plate - Context Size $5$}
    \end{subfigure}
    \hfill % Horizontal spacing between subfigures
    \begin{subfigure}[b]{0.49\linewidth} % Adjust the width as needed
        \includegraphics[width=\textwidth]{03_appendix/figure_matrix/mse_time_steps/planar_bending/mse_per_timestep_2fig_context_size_2.pdf}
        \caption{Planar Bending - Context Size $2$}
    \end{subfigure}
    \begin{subfigure}[b]{0.49\linewidth} % Adjust the width as needed
        \includegraphics[width=\textwidth]{03_appendix/figure_matrix/mse_time_steps/teddy_fall_nopc/mse_per_timestep_2fig_context_size_20.pdf}
        \caption{Falling Teddy Bear - Context Size $20$}
    \end{subfigure}
    \hfill % Horizontal spacing between subfigures
    \begin{subfigure}[b]{0.49\linewidth} % Adjust the width as needed
        \includegraphics[width=\textwidth]{03_appendix/figure_matrix/mse_time_steps/multi_objects_fall_varied_material/mse_per_timestep_2fig_context_size_20.pdf}
        \caption{Multi Objects Fall - Context Size $20$}
    \end{subfigure}
    \caption{
    \rebuttal{\glsfirst{mse} over timesteps for varied tasks. Overall, autoregressive methods suffer from accumulated errors, while using \gls{prodmp} as a trajectory representation, \model results in lower MSE across timesteps.}}
    \vspace{-0.3cm}
    \label{fig:mse_timestep_all_4}
\end{figure*}
