# Supplementary material for: Context-aware Learned Mesh-based Simulation via Trajectory-Level Meta-Learning
Source: arXiv:2511.05234 source file (2026-01-21)
Supplement: Supplementary file 4 [file figure_runtime_evaluation_gth_tikzplotlib.tex]

% This file was created with tikzplotlib v0.10.1.
\begin{tikzpicture}

\definecolor{darkgray}{RGB}{169,169,169}
\definecolor{darkgray176}{RGB}{176,176,176}
\definecolor{darkorange25512714}{RGB}{255,127,14}
\definecolor{forestgreen4416044}{RGB}{44,160,44}
\definecolor{lightgray204}{RGB}{204,204,204}
\definecolor{steelblue31119180}{RGB}{31,119,180}

\begin{axis}[
width=0.54\textwidth,
axis line style={darkgray},
legend cell align={left},
legend style={
  fill opacity=0.95,
  draw opacity=1,
  text opacity=1,
  at={(0.025,0.975)},
  anchor=north west,
  draw=lightgray204,
  font=\fontsize{9}{11}\selectfont,
},
log basis y={10},
tick align=outside,
tick pos=left,
x grid style={darkgray176},
xmin=0.5, xmax=11,
xtick style={color=darkgray},
xtick={2,4.5,7,9.5},
xticklabel style={font=\fontsize{9}{11}\selectfont},
xticklabels={Deformable Block,Sheet Deformation,Tissue Manipulation,Mixed Obj. Falling},
xmajorgrids,
xticklabel style={rotate=45.0},
y grid style={darkgray176},
ylabel={Inference Time $[s]$},
ylabel style={font=\fontsize{9}{11}\selectfont}, 
ymajorgrids,
ymin=1e-3, ymax=25,
log origin=infty,
ymode=log,
ytick style={color=darkgray},
ytick={0.001,0.01,0.1,1,10,100},
yticklabels={
  \(\displaystyle {0.001}\),
  \(\displaystyle {0.01}\),
  \(\displaystyle {0.1}\),
  \(\displaystyle {1}\),
  \(\displaystyle {10}\),
  \(\displaystyle {100}\)
},
ybar, % Enable bar plot style
bar width=0.4 % Optional: Adjust bar width
]

% Data for steelblue
\addplot+[
  color=steelblue31119180,
  fill=steelblue31119180
] coordinates {
  (1.85, 0.03)
  (4.35, 0.032)
  (6.85, 0.089)
  (9.35, 0.04)
};

% Data for darkorange
\addplot+[
  color=darkorange25512714,
  fill=darkorange25512714
] coordinates {
  (2, 0.255)
  (4.5, 0.28)
  (7, 0.64)
  (9.5, 1.36)
};

% Data for forestgreen
\addplot+[
  color=forestgreen4416044,
  fill=forestgreen4416044
] coordinates {
  (2.15, 1)
  (4.65, 14)
  (7.15, 5)
  (9.65, 2)
};

\end{axis}

\end{tikzpicture}
