# Supplementary material for: Context-aware Learned Mesh-based Simulation via Trajectory-Level Meta-Learning
Source: arXiv:2511.05234 source file (2026-01-21)
Supplement: Supplementary file 5 [file figure_runtime_evaluation_tikzplotlib.tex]

% This file was created with tikzplotlib v0.10.1.
\begin{tikzpicture}

\definecolor{darkgray}{RGB}{169,169,169}
\definecolor{darkgray176}{RGB}{176,176,176}
\definecolor{darkorange25512714}{RGB}{255,127,14}
\definecolor{lightgray204}{RGB}{204,204,204}
\definecolor{steelblue31119180}{RGB}{31,119,180}

\begin{axis}[
height=6.5cm,
axis line style={darkgray},
legend cell align={left},
legend style={
  fill opacity=0.95,
  draw opacity=1,
  text opacity=1,
  at={(0.025,0.975)},
  anchor=north west,
  draw=lightgray204,
  font=\fontsize{9}{11}\selectfont,
},
tick align=outside,
tick pos=left,
x grid style={darkgray176},
xmin=-0.865, xmax=12,
xmajorticks=true,
xtick style={draw=none},
xtick={0,2.5,5,7.5,10.0},
xticklabel style={rotate=45.0, font=\fontsize{9}{11}\selectfont},
xticklabels={Deformable Block,Sheet Deformation,Tissue Manipulation,Falling Teddy Bear, Mixed Obj. Falling},
y grid style={darkgray176},
ylabel={Inference Time $[s]$},
ylabel style={font=\fontsize{9}{11}\selectfont},  % Change font size here
ymajorgrids,
ymin=0, ymax=1.428,
ytick style={color=darkgray},
ytick={0, 0.25, 0.5, 0.75, 1.0, 1.25},
]
% Define blue for M3GN (Ours) and orange for MGN in the legend using predefined colors
\addlegendimage{area legend, fill=steelblue31119180}
\addlegendentry{\textbf{M3GN} (Ours)}
\addlegendimage{area legend, fill=darkorange25512714}
\addlegendentry{MGN}
\draw[draw=none,fill=steelblue31119180] (axis cs:-0.4,0) rectangle (axis cs:0.4,0.03);
\draw[draw=none,fill=darkorange25512714] (axis cs:0.6,0) rectangle (axis cs:1.4,0.255);
\draw[draw=none,fill=steelblue31119180] (axis cs:2.1,0) rectangle (axis cs:2.9,0.032);
\draw[draw=none,fill=darkorange25512714] (axis cs:3.1,0) rectangle (axis cs:3.9,0.28);
\draw[draw=none,fill=steelblue31119180] (axis cs:4.6,0) rectangle (axis cs:5.4,0.089);
\draw[draw=none,fill=darkorange25512714] (axis cs:5.6,0) rectangle (axis cs:6.4,0.64);
\draw[draw=none,fill=steelblue31119180] (axis cs:7.1,0) rectangle (axis cs:7.9,0.04);
\draw[draw=none,fill=darkorange25512714] (axis cs:8.1,0) rectangle (axis cs:8.9,1.36);
\draw[draw=none,fill=steelblue31119180] (axis cs:9.6,0) rectangle (axis cs:10.4,0.04);
\draw[draw=none,fill=darkorange25512714] (axis cs:10.6,0) rectangle (axis cs:11.4,1.36);
\end{axis}

\end{tikzpicture}
