# Supplementary material for: Context-aware Learned Mesh-based Simulation via Trajectory-Level Meta-Learning
Source: arXiv:2511.05234 source file (2026-01-21)
Supplement: Supplementary file 6 [file runtime_evaluation.tex]

% \begin{figure}
%     \centering
%     \input{03_appendix/figure_runtime_evaluation_tikzplotlib}    
%     \caption{Runtime comparison between \gls{ltsgns} and \gls{mgn} on all tasks with a context size of $10$. Including the cost of predicting the latent task descriptions from the provided contexts, \gls{ltsgns} is up to 32 times faster than~\gls{mgn} while improving simulation accuracy.}
%     \label{fig:enter-label}
% \end{figure}

\begin{figure}  % 'r' for right alignment; adjust width as needed
    \centering
    \begin{tikzpicture}
        \definecolor{darkgray}{RGB}{169,169,169}
        \definecolor{darkgray176}{RGB}{176,176,176}
        \definecolor{darkorange25512714}{RGB}{255,127,14}
        \definecolor{forestgreen4416044}{RGB}{44,160,44}
        \definecolor{lightgray204}{RGB}{204,204,204}
        \definecolor{steelblue31119180}{RGB}{31,119,180}
        \tikzstyle{every node}=[font=\scriptsize]
        \input{tikz_colors}
        \begin{axis}[%
        hide axis,
        xmin=10,
        xmax=50,
        ymin=0,
        ymax=0.1,
        legend style={
            draw=none,
            legend cell align=left,
            legend columns=3, % Adjust columns to fit all entries
            column sep=1ex,   % Space between columns
            font=\huge, % Adjust font size for the legend
        },
        ]
        % Add legend images with ybar style
        \addlegendimage{area legend, fill=steelblue31119180}
        \addlegendentry{\textbf{M3GN} (Ours)}
        \addlegendimage{area legend, fill=darkorange25512714}
        \addlegendentry{MGN}
        \addlegendimage{area legend, fill=forestgreen4416044}
        \addlegendentry{Gth. Simulation}
        \end{axis}
    \end{tikzpicture}

    \input{03_appendix/figure_runtime_evaluation_gth_tikzplotlib}    
    \caption{\rebuttal{Runtime comparison between \gls{ltsgns} and \gls{mgn}, and the corresponding ground truth simulator on all tasks. Note the log-scale of the y-axis. Including the cost of predicting the latent task descriptions from the provided contexts, \gls{ltsgns} is up to 32 times faster than~\gls{mgn} and up to 400 times faster than a traditional simulator.}     
    }
    \label{fig:runtime}
\end{figure}

% \begin{figure}[t!]
%     \centering
    
%     
%     \label{fig:runtime}
% \end{figure}
